# Supplementary material for: Concept Distillation: Leveraging Human-Centered Explanations for Model Improvement
Source: arXiv:2311.15303 source file (2023-11-26)
Supplement: Supplementary file 1 [file appendix.tex]

% \clearpage\appendix
\section{Appendix}
\subsection{RRR loss}
RRR \cite{schramowski2020making} has a reasoning loss which is added to the original GT loss of a classifier with a factor $\lambda$ and is is given as:
$$
\begin{aligned}
Loss_{RRR} = \underbrace{ \sum_{n=1}^N \sum_{d=1}^D\left(A_{n d} \frac{\partial}{\partial x_{n d}} \sum_{k=1}^K \log \left(\hat{y}_{n k}\right)\right)^2}_{\text {Right reasons }}
\end{aligned}
$$
Where $A \in\{0,1\}^{N \times D}$is the user provided annotation matrix which is a binary mask telling whether dimension $D$ should be irrelevant for prediction of observation $n$. RRR thus penalises the gradients over the binary mask feature-wise for each input sample and is a local XAI method. We use this loss for encorportating local knowledge in our system.
In case of debiasing color concept we take the programitc rule of single pixel not affecting (single pixel represents color information) while a group of pixels affecting as demonstrated by \cite{rieger2020interpretations} for their adaptation of RRR. Note that since RRR is a local XAI method we cannot use this loss over BFFHQ since it cannot encode age since  pixel-wise annotations for such complex concepts are near-impossible. We thus show its application in MNIST datasets wherein color or texture are the biases.

\subsection{Implementation Details}
In our experiments, we use a logistic regression implemented by a single perceptron layer with sigmoid activation trained with cross-entropy loss for binary classification (between positive and negative concept set images). We use DINO \cite{caron2021emerging } as a teacher which gives 778 dimentional feature image which is reduced to 64 by applying PCA over it. 
We use two convolution layers followed by 2 fully connected layer network for MNIST experiments as done by \cite{rieger2020interpretations} \cite{lee2021learning}. We apply concept distillation in the second convolution layer here. 
We use Resnet18 (no pre-training) architecture for BFFHQ as done by \cite{lee2021learning} and apply our method over "layer4.1.conv1" layer. We use Adam \cite{kingma2014adam} optimizer with a learning rate of 10e-4 and beta being in range 0.9 to 0.999 and ep of 1e-08 with a weight decay of 0 (all default pytorch values except learning late). We use a batch size of 32 for MNIST experiments and 64 for BFFHQ experiments.
For mapping module we use 1 up-convolution and 1 down-convolution layer for encoder and decoders. We train the autoencoders with an L2 loss. 

For training the MNIST and BFFHQ models we use cross entropy loss as GT loss and our loss given in \autoref{eqn:LC} as our concept loss weighted by a parameter $\lambda L_C$ which was varied from 0.01 to 10e5 and its found to work best for values close to 20 for MNIST datasets. Other parameter values which we found to work best:  $k = 7$, $\alpha = 0.3$, we found  number of images in concept set to work best with 150 images for ColorMNIST.

% \subsection{Details of DINO}

\subsection{Dataset set details}
\subsubsection{MNIST datasets}
We show the bias in the various MNIST datasets in \autoref{fig:biased_datasets}.
For MNIST datasets (ColorMNIST and DecoyMNIST) we use the splits by \cite{rieger2020interpretations}. For the creation of TextureMNIST, we use the above-obtained splits of digits and use DTD \cite{cimpoi2014describing} dataset for obtaining textures.
%We simply multiply the digits with random textures chosen from DTD dataset.
We use random flat colored patches as concept "color" and random textures(not used in training/test set) in "textures" concept. We use gray colored patches as "gray" concept set.
For negative concept set we create random shaped white blobs in black background.

We show our Pixel Hard MNIST test set in \autoref{fig:pixel_hard}.

\subsubsection{BFFHQ Details}
We take the 48 images each for young men and old women (Non-biased examples) concepts as given by \cite{lee2021learning} in their adversarial images while we sample 48-48 images from trainset to form biased examples concept sets of young women and old men. We use the same train-test-validation split as done by \cite{lee2021learning}.

In our experiments, we define "old" concept set as images of both men and women who are old while the "young" concept set as having young men and women and "mix" having both men and women of all ages.

\subsubsection{IID Details}
We use the same model and same training datasets as done by \cite{CGintrinsics}. We also use the same losses( IIW loss, GT loss, SAW loss) and add our Concept loss over the last layer of CGIID model training for 5-15 epochs.
We demonstrate our IID concept sets in \autoref{appendix:iid_concepts}.

\begin{figure}[t]
    \centering
    \includegraphics[width=0.43\textwidth]{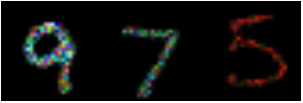}
    % \vspace{-1pt}
    \caption{pixel hard MNIST test set}
    \label{fig:pixel_hard}
\end{figure}

\begin{figure}[t]
    \centering
    \includegraphics[width=\linewidth, height=5cm]{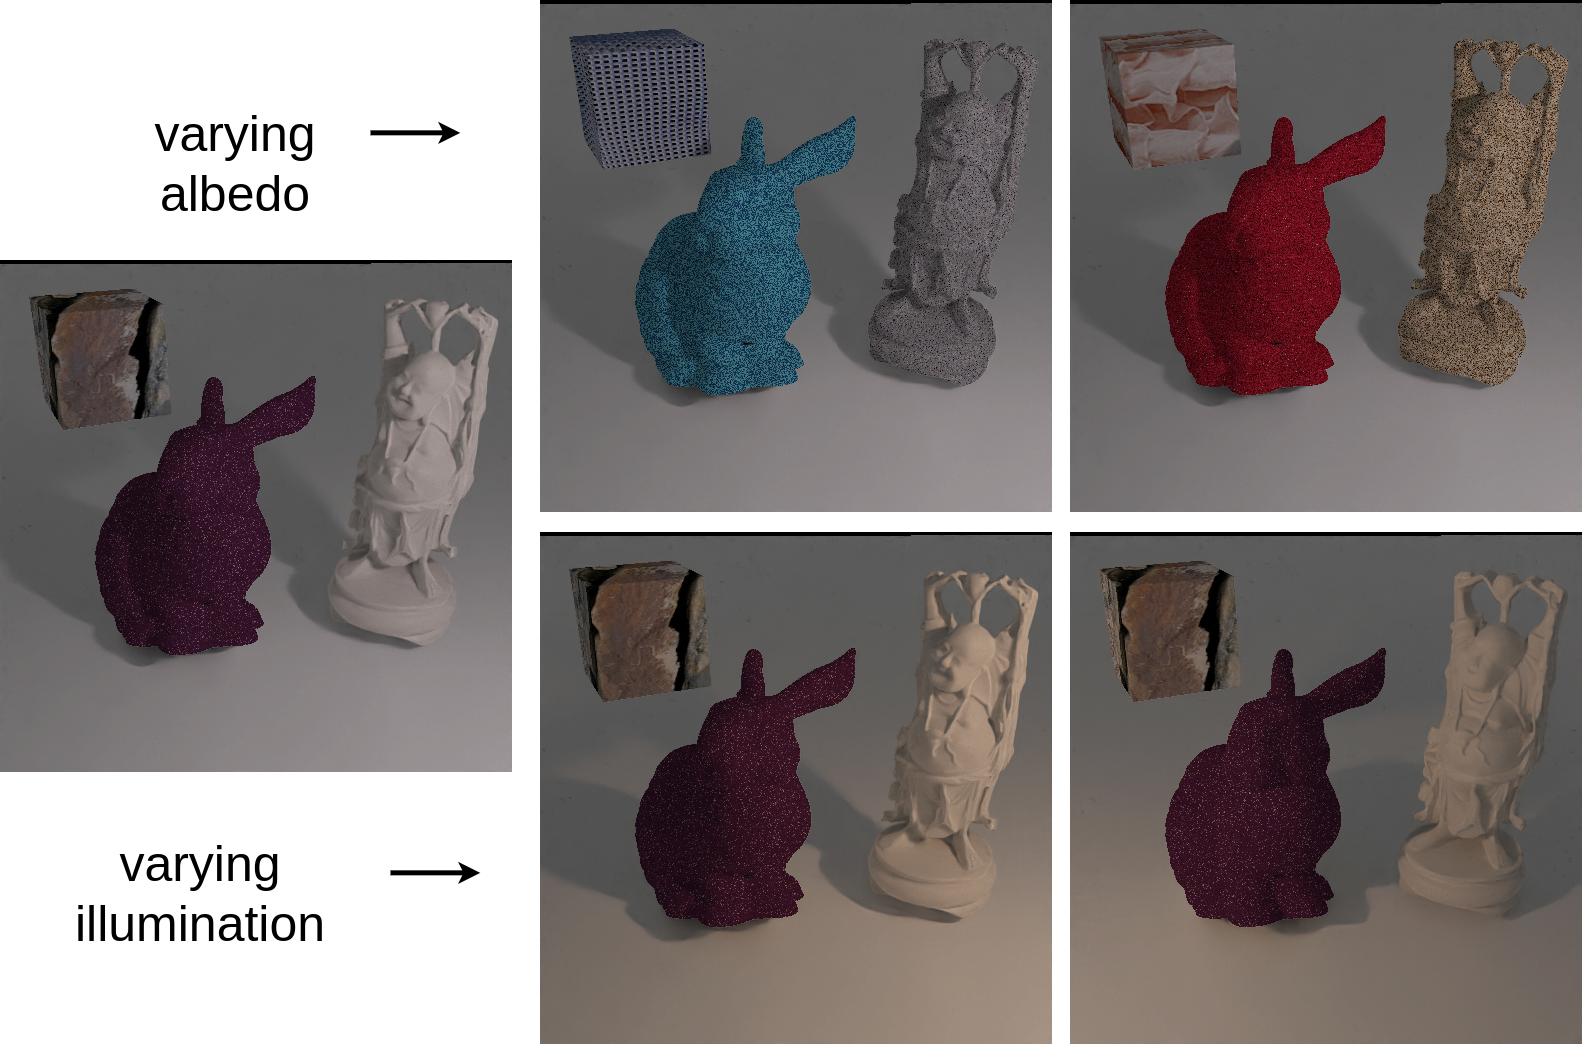}
    % \vspace{-1pt}
    \caption{Concept sets used for IID experiments}
    \label{appendix:iid_concepts}
\end{figure}

\subsection{Additional Results}
We show the additional IID results in \autoref{fig:IID_res_more}. It can be seen that our method is able to remove the illumination information from it and flatten the predictions of R ($\hat R$) as well.
% \subsection{Concept Set details}
% \input{figures/IIDconcepts.tex}
% We provide the details of our concept sets used for IID in \autoref{fig:IIDconepts}.
% % \subsection{Algorithm}
% % \label{appendix:Algorithm}
\
\begin{figure*}
    \centering
    \includegraphics[width=\textwidth]{assets/results/IID_res_all.jpg}
    \caption{Qualitative IID results: Our method is able to make the $\hat R$ less sensitive to illumination (thereby removing the concept of illumination from $\hat R$ and during this $\hat R$ predictions become more flat without specifically introducing the flatness prior suggesting disentanglement of R-S is a better way to improve IID. Also the illumination information removed from $\hat R$ is introduced in $\hat S$. }
    \label{fig:IID_res_more}\vspace*{-3mm}
\end{figure*}

% \subsection{CDEP+RRR}
% \subsection{clevr-hans}
% \subsection{Extra results} 
% TextureMNIST dataset 10 imgs. 
% GradCams for all digits/faces 
% IID extra results

% \subsection{IID concept sets rendering}
